# Supplementary material for: Bayesian Metric Learning for Uncertainty Quantification in Image Retrieval
Source: arXiv:2302.01332 source file (2023-02-04)
Supplement: Supplementary file 1 [file 07new_appendix.tex]

\subsection{Probabilistic view of the contrastive loss.}\label{sec:prob_contrastive} The contrastive loss \cref{eq:contrastive_definition} attracts positive pairs and repels negative pairs by minimizing an MSE loss between the positives and maximizing the MSE loss between the negatives \cref{eq:contrastive_definition}. Minimizing the positive term is equivalent to maximizing an isotropic Gaussian log-likelihood, whereas maximizing the negative term corresponds to maximizing an isotropic "reversed" Gaussian log-likelihood. Due to the $l2$ normalization that makes the latent space compact, this "reversed" Gaussian distribution is well defined. This implies that the contrastive loss is indeed a proper log-posterior distribution.
