# Supplementary material for: Bayesian Metric Learning for Uncertainty Quantification in Image Retrieval
Source: arXiv:2302.01332 source file (2023-02-04)
Supplement: Supplementary file 2 [file 07old_appendix.tex]

\subsection{Probabilistic view of the contrastive loss.}\label{sec:prob_contrastive} The contrastive loss \cref{eq:contrastive_definition} attracts positive pairs and repels negative pairs by minimizing an MSE loss between the positives and maximizing the MSE loss between the negatives \cref{eq:contrastive_definition}. Minimizing the positive term is equivalent to maximizing an isotropic Gaussian log-likelihood, whereas maximizing the negative term corresponds to maximizing an isotropic "reversed" Gaussian log-likelihood. Due to the $\ell^2$-normalization that makes the latent space compact, this "reversed" Gaussian distribution is well defined. This implies that the contrastive loss is indeed a proper log-posterior distribution. 


\begin{table*}
    \centering
    \resizebox{\textwidth}{!}{\begin{tabular}{cccccccccccc}
    &   R@1    &   R@5    &   R@10    &   R@20    &   M@5    &   M@10    &   M@20    &   AUROC    &   AUPRC    &   AUSC    &   ECE\\ \hline
deterministic & $0.78\pm0.01$ & $0.93\pm0.0$ & $0.96\pm0.0$ & $0.98\pm0.0$ & $0.73\pm0.01$ & $0.72\pm0.01$ & $0.71\pm0.01$ & $-$ & $-$ & $-$ & $-$ \\
pfe & $0.79\pm0.01$ & $0.93\pm0.0$ & $0.96\pm0.0$ & $0.98\pm0.0$ & $0.74\pm0.01$ & $0.72\pm0.01$ & $0.71\pm0.01$ & $0.69\pm0.11$ & $0.64\pm0.1$ & $0.83\pm0.04$ & $0.19\pm0.03$ \\
laplace posthoc fix & $0.78\pm0.01$ & $0.93\pm0.0$ & $0.96\pm0.0$ & $0.98\pm0.0$ & $0.74\pm0.01$ & $0.72\pm0.01$ & $0.71\pm0.01$ & $0.96\pm0.01$ & $0.96\pm0.01$ & $0.85\pm0.02$ & $0.04\pm0.0$ \\
laplace posthoc pos & $0.79\pm0.01$ & $0.93\pm0.0$ & $0.96\pm0.0$ & $0.98\pm0.0$ & $0.74\pm0.01$ & $0.72\pm0.01$ & $0.71\pm0.01$ & $0.98\pm0.01$ & $0.98\pm0.01$ & $0.78\pm0.02$ & $0.05\pm0.01$ \\
laplace posthoc full & $0.79\pm0.01$ & $0.93\pm0.0$ & $0.96\pm0.0$ & $0.98\pm0.0$ & $0.74\pm0.01$ & $0.72\pm0.01$ & $0.71\pm0.01$ & $0.95\pm0.01$ & $0.95\pm0.01$ & $0.82\pm0.01$ & $0.03\pm0.0$ \\
laplace online fix & $0.81\pm0.0$ & $0.94\pm0.0$ & $0.96\pm0.0$ & $0.98\pm0.0$ & $0.77\pm0.0$ & $0.76\pm0.0$ & $0.75\pm0.0$ & $0.97\pm0.02$ & $0.97\pm0.02$ & $0.9\pm0.01$ & $0.03\pm0.0$ \\
laplace online pos & $0.81\pm0.01$ & $0.94\pm0.0$ & $0.96\pm0.0$ & $0.98\pm0.0$ & $0.78\pm0.0$ & $0.77\pm0.0$ & $0.76\pm0.0$ & $0.96\pm0.02$ & $0.96\pm0.03$ & $0.84\pm0.03$ & $0.44\pm0.02$ \\
laplace online full & $0.81\pm0.0$ & $0.94\pm0.0$ & $0.96\pm0.0$ & $0.98\pm0.0$ & $0.77\pm0.0$ & $0.76\pm0.0$ & $0.75\pm0.01$ & $0.97\pm0.01$ & $0.97\pm0.01$ & $0.85\pm0.01$ & $0.02\pm0.0$ \\
laplace posthoc arccos pos & $0.79\pm0.01$ & $0.93\pm0.0$ & $0.96\pm0.0$ & $0.98\pm0.0$ & $0.74\pm0.01$ & $0.72\pm0.01$ & $0.71\pm0.01$ & $0.92\pm0.01$ & $0.89\pm0.02$ & $0.71\pm0.01$ & $0.06\pm0.01$ \\
laplace posthoc arccos full & $0.79\pm0.01$ & $0.93\pm0.0$ & $0.96\pm0.0$ & $0.98\pm0.0$ & $0.74\pm0.01$ & $0.72\pm0.01$ & $0.71\pm0.01$ & $0.92\pm0.02$ & $0.89\pm0.03$ & $0.73\pm0.02$ & $0.02\pm0.0$ \\
laplace online arccos pos & $0.82\pm0.01$ & $0.94\pm0.0$ & $0.96\pm0.0$ & $0.98\pm0.0$ & $0.78\pm0.01$ & $0.76\pm0.01$ & $0.76\pm0.0$ & $0.97\pm0.01$ & $0.96\pm0.02$ & $0.83\pm0.04$ & $0.33\pm0.13$ \\
laplace online arccos full & $0.82\pm0.0$ & $0.94\pm0.0$ & $0.96\pm0.0$ & $0.98\pm0.0$ & $0.78\pm0.0$ & $0.77\pm0.0$ & $0.76\pm0.0$ & $0.96\pm0.01$ & $0.96\pm0.01$ & $0.8\pm0.01$ & $0.21\pm0.04$ \\
    \end{tabular}}
    \caption{Caption}
    % \label{tab:my_label}
\end{table*}



\section{Full results}

\begin{table*}
    \centering
    \resizebox{\textwidth}{!}{\begin{tabular}{cccccccccccc}
    &   R@1    &   R@5    &   R@10    &   R@20    &   M@5    &   M@10    &   M@20    &   AUROC    &   AUPRC    &   AUSC    &   ECE\\
deterministic & $0.61\pm0.01$ & $0.83\pm0.0$ & $0.89\pm0.0$ & $0.94\pm0.0$ & $0.48\pm0.0$ & $0.41\pm0.0$ & $0.34\pm0.0$ & $-$ & $-$ & $-$ & $-$ \\
pfe & $0.63\pm0.01$ & $0.85\pm0.01$ & $0.91\pm0.0$ & $0.94\pm0.0$ & $0.5\pm0.0$ & $0.43\pm0.0$ & $0.36\pm0.0$ & $0.32\pm0.19$ & $0.46\pm0.07$ & $0.62\pm0.01$ & $0.1\pm0.01$ \\
laplace posthoc fix & $0.94\pm0.0$ & $0.99\pm0.0$ & $0.99\pm0.0$ & $1.0\pm0.0$ & $0.91\pm0.0$ & $0.88\pm0.0$ & $0.83\pm0.0$ & $0.52\pm0.04$ & $0.6\pm0.02$ & $0.93\pm0.0$ & $0.23\pm0.01$ \\
laplace posthoc pos & $0.94\pm0.0$ & $0.99\pm0.0$ & $0.99\pm0.0$ & $1.0\pm0.0$ & $0.9\pm0.0$ & $0.88\pm0.0$ & $0.83\pm0.0$ & $0.53\pm0.04$ & $0.6\pm0.03$ & $0.93\pm0.01$ & $0.22\pm0.02$ \\
laplace posthoc full & $0.94\pm0.0$ & $0.99\pm0.0$ & $0.99\pm0.0$ & $1.0\pm0.0$ & $0.9\pm0.0$ & $0.88\pm0.0$ & $0.83\pm0.0$ & $0.52\pm0.04$ & $0.6\pm0.02$ & $0.93\pm0.01$ & $0.23\pm0.01$ \\
laplace online fix & $0.93\pm0.0$ & $0.99\pm0.0$ & $1.0\pm0.0$ & $1.0\pm0.0$ & $0.88\pm0.0$ & $0.85\pm0.0$ & $0.8\pm0.0$ & $0.5\pm0.02$ & $0.59\pm0.02$ & $0.92\pm0.01$ & $0.17\pm0.01$ \\
laplace online pos & $0.93\pm0.0$ & $0.99\pm0.0$ & $0.99\pm0.0$ & $1.0\pm0.0$ & $0.88\pm0.0$ & $0.85\pm0.0$ & $0.8\pm0.0$ & $0.46\pm0.1$ & $0.56\pm0.06$ & $0.92\pm0.01$ & $0.17\pm0.0$ \\
laplace online full & $0.93\pm0.0$ & $0.99\pm0.0$ & $0.99\pm0.0$ & $1.0\pm0.0$ & $0.88\pm0.0$ & $0.85\pm0.0$ & $0.8\pm0.0$ & $0.42\pm0.08$ & $0.53\pm0.05$ & $0.92\pm0.01$ & $0.17\pm0.01$ \\
laplace posthoc arccos pos & $0.94\pm0.0$ & $0.99\pm0.0$ & $0.99\pm0.0$ & $1.0\pm0.0$ & $0.9\pm0.0$ & $0.88\pm0.0$ & $0.83\pm0.0$ & $0.58\pm0.1$ & $0.6\pm0.08$ & $0.92\pm0.01$ & $0.22\pm0.01$ \\
laplace posthoc arccos full & $0.94\pm0.0$ & $0.99\pm0.0$ & $0.99\pm0.0$ & $1.0\pm0.0$ & $0.9\pm0.0$ & $0.88\pm0.0$ & $0.83\pm0.0$ & $0.56\pm0.11$ & $0.61\pm0.09$ & $0.93\pm0.01$ & $0.23\pm0.01$ \\
laplace online arccos pos & $0.92\pm0.0$ & $0.99\pm0.0$ & $0.99\pm0.0$ & $1.0\pm0.0$ & $0.87\pm0.0$ & $0.84\pm0.0$ & $0.78\pm0.0$ & $0.55\pm0.1$ & $0.63\pm0.08$ & $0.92\pm0.01$ & $0.18\pm0.01$ \\
laplace online arccos full & $0.92\pm0.0$ & $0.99\pm0.0$ & $0.99\pm0.0$ & $1.0\pm0.0$ & $0.88\pm0.0$ & $0.85\pm0.0$ & $0.8\pm0.0$ & $0.45\pm0.06$ & $0.55\pm0.04$ & $0.91\pm0.0$ & $0.19\pm0.02$ \\
    \end{tabular}}
    \caption{Caption}
    % \label{tab:my_label}
\end{table*}












\section{Method (old)}

Let $\mathcal{X}$ be the data space, $\mathcal{Z}$ be the latent space, $\Theta$ be the parameter space. For a given neural network architecture $f$ and a parameter vector $\theta\in\Theta$, $f_\theta$ is a function
\begin{equation}
f_\theta: \mathcal{X} \rightarrow \mathcal{Z}
\end{equation}
The discrete set $\mathcal{C}=\{c_i\}_{i=1,\dots,C}$ of classes induces a partition of the points in the data space. A dataset is a collection of pairs datapoint-class $(x,c)\in\mathcal{X}\times\mathcal{C}$.
\begin{equation}
\mathcal{D} = \{(x_i,c_i)\}_{i=1,\dots,D}
\end{equation}

We assume that every dataset contains at least one element for each class. This assumption, excluding from $\mathcal{C}$ the classes that never appear, is equivalent to
\begin{equation}\label{assumption:no_empty_class}
    \{(x_i,c_i)\in\mathcal{D}_1 | c_i = c\}
    \not=
    \emptyset
    \iff
    \{(x_i,c_i)\in\mathcal{D}_2 | c_i = c\}
    \not=
    \emptyset
    \qquad \forall c\in\mathcal{C}
\end{equation}

The margin $m\in\mathbb{R}$ is a positive fixed constant.


\subsection{Classic non-probabilistic view}
Given a pair of datapoints $(x_e,c_e),(x_a,c_a)\in\mathcal{D}$, we can define the contrastive loss as
\begin{equation}\label{eq:contrastive_definition}
    \text{contrastive}(\theta;x_e,c_e,x_a,c_a)
    =
    \begin{cases}
        \frac{1}{2}\|f_\theta(x_e)-f_\theta(x_a)\|^2 & \text{if } c_e=c_a \\
        \frac{1}{2}\max(-\|f_\theta(x_e)-f_\theta(x_a)\|^2 + m,0)  & \text{if } c_e\not=c_a
    \end{cases}
\end{equation}
and then we can define the loss as the sum of the contrastive on all possible pairs
\begin{equation}
    \text{loss}(\theta;\mathcal{D})
    =
    \sum_{((x_e,c_e),(x_a,c_a))\in\mathcal{D}^2}\text{contrastive}(\theta;x_e,c_e,x_a,c_a)
\end{equation}

Notice that the contrastive term is symmetric with respect to a switch of datapoints in a pair. Also notice that the contrastive term of a datapoint with itself is 0, as the embedding $f_\theta(x)$ is the same. Thus, up to a factor 2, the loss can equivalently be defined as a sum over ordered pairs.


\subsection{Probabilistic view}
In the metric learning framework, a dataset $\mathcal{D}$ plays two very different roles at the same time. This happens in the same spirit as, in electrostatics, a charged particle at the same time \emph{generates} an electric field and \emph{interact} with the existing electric field. This subtle difference, although being neglectable in the classic setting, is conceptually important in the probabilistic setting. Thus, for now, we assume to be given an \emph{anchor} dataset $\mathcal{D}_A$ and an \emph{evaluation} dataset $\mathcal{D}_E$. Only after the derivations we will set them to be equal.

The \textbf{anchor} dataset $\mathcal{D}_A$ induces a scalar-valued function $p^c_{\mathcal{Z}}\in\Delta(\mathcal{Z)}$ on the latent space for each class $c\in\mathcal{C}$. This function is given by
\begin{equation}\label{eq:induced_distribution_definition}
    p^c_{\mathcal{Z}}(z|\mathcal{D}_A,\theta)
    =
    \prod_{\substack{(x_i,c_i)\in\mathcal{D}_A \\ \text{s.t. } c_i = c}}
    p^{\shortrightarrow\shortleftarrow}(z|x_i,\theta)
    \prod_{\substack{(x_i,c_i)\in\mathcal{D}_A \\ \text{s.t. } c_i\not= c}}
    p^{\shortleftarrow\shortrightarrow}(z|x_i,\theta)
\end{equation}
that is a product of one \emph{attractive distribution} term $p^{\shortrightarrow\shortleftarrow}$ for all anchor points of the same class, times a \emph{repulsive distribution} term $p^{\shortleftarrow\shortrightarrow}$ for all anchor points of different classes. This product of distributions is not a distribution itself (sigh). Actually it is a normalizable function, but the normalization constant depends on $\theta$ and this dependency breaks everything in the following (gradients are not equivalent in the two settings), so we must stick with this non-distribution function.

We can define the log density of the attractive term as
\begin{equation}\label{eq:log_attractive_definition}
    \log p^{\shortrightarrow\shortleftarrow}(z|x,\theta)
    :=
    -\frac{1}{2} \|z - f_\theta(x)\|^2
    +
    c^{\shortrightarrow\shortleftarrow}
\end{equation}
and the log "density" of the repulsive term as
\begin{equation}\label{eq:log_repulsive_definition}
    \log p^{\shortleftarrow\shortrightarrow}(z|x,\theta)
    :=
    \min\left(\frac{1}{2}\|z - f_\theta(x)\|^2- \frac{m}{2},0\right)
    +
    c^{\shortleftarrow\shortrightarrow}.
\end{equation}
Up to some normalizing constant, the attractive term is a Gaussian distribution centered in $f_\theta(x)$
\begin{equation}
    p^{\shortrightarrow\shortleftarrow}(z|x,\theta)
    \sim \mathcal{N}(z| \mu=f_\theta(x), \Sigma=\mathbb{I})
\end{equation}
and similarly, the repulsive term is a "reversed and cropped" Gaussian, which we can write as
\begin{equation}
    p^{\shortleftarrow\shortrightarrow}(z|x,\theta)
    \sim \reflectbox{$\mathcal{N}$}(z| \mu=f_\theta(x), \Sigma=\mathbb{I}, m).
\end{equation}
It's important to notice at this point that if we make no further assumption on the latent space $\mathcal{Z}$, the repulsive term $p^{\shortleftarrow\shortrightarrow}$, as defined in \cref{eq:log_repulsive_definition}, is not normalizable. Thus it is not a proper distribution on $\mathcal{Z}$. But that does not mean that this abstract quantity is of no use to us. For it plays a mathematical role that is entirely independent of the probabilistic interpretation.\\
In fact, under the no-empty-class dataset assumption (\ref{assumption:no_empty_class}), it is guaranteed that the overall product $p^c_{\mathcal{Z}}$ is normalizable. Thus it preserves the probabilistic interpretation of distribution induced by an anchor dataset.

Yet this can be unsatisfactory for most readers. If, instead, we choose the manifold $\mathcal{Z}$ to be \emph{compact} (and submanifold of $\mathbb{R}^D$, but please why shouldn't you) then it has finite measure and $p^{\shortleftarrow\shortrightarrow}$ is guaranteed to be normalizable, thus it is actually a "reversed Gaussian \emph{distribution}".\\
Note that the addition of the $l^2$-normalization layer at the end of a NN is one way of choosing $\mathcal{Z}=\mathcal{S}^n$, the unit sphere, a compact submanifold of $\mathbb{R}^{n+1}$.\\ (TODO: fix this setting, smash the head on the integral and compute the normalization constants.)

\fred{Can we make a visualization of this "reversed Gaussian"? I think by drawing it, it is much easier to conceptualize. Maybe just add a hand-drawn sketch to begin with.  }

\begin{figure}[th!]
    \centering
    \includegraphics[width=0.5\textwidth]{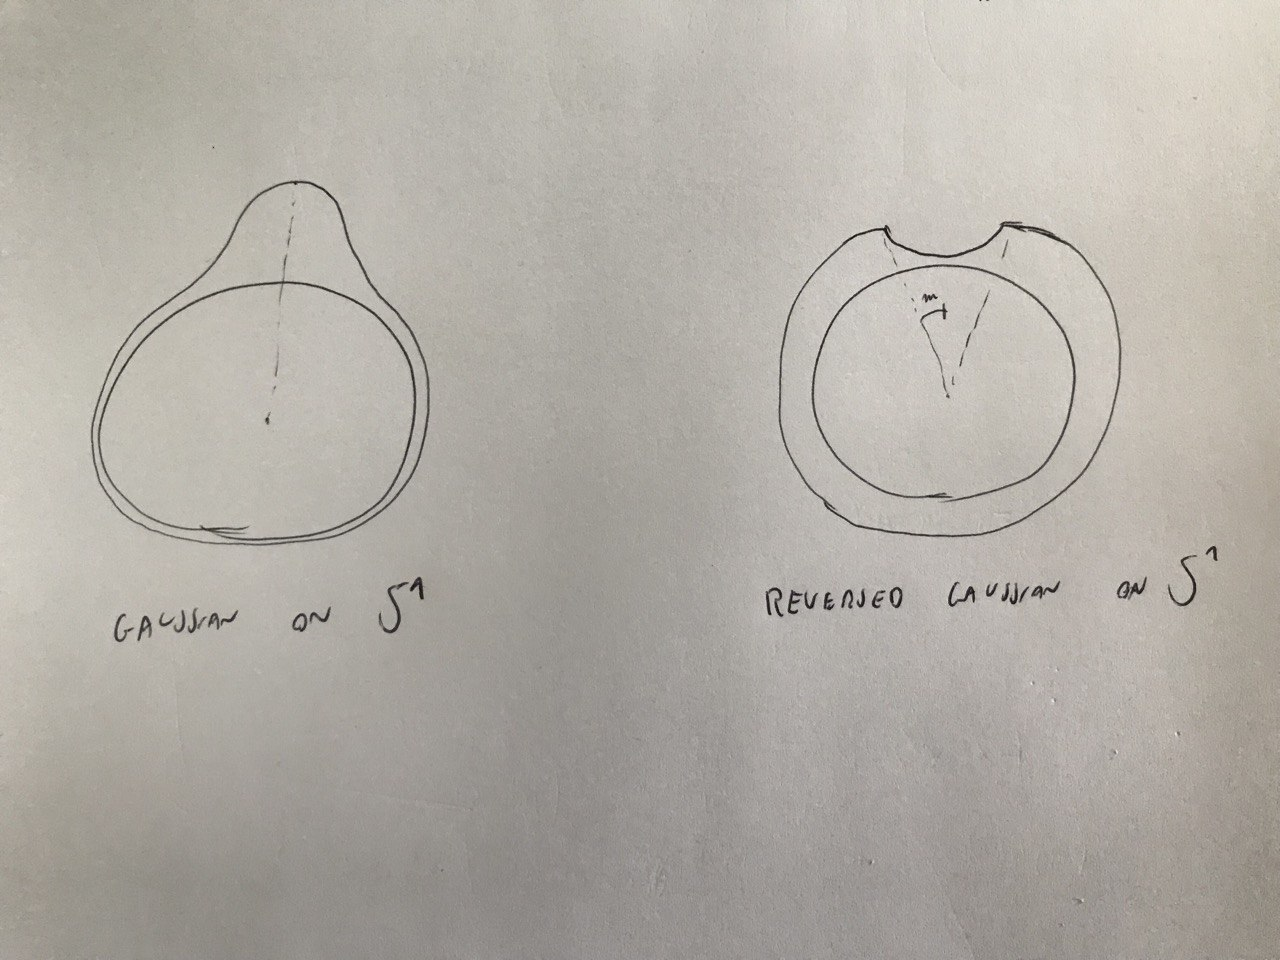}
    \caption{\textbf{Reversed Gaussian visualization.} This is tricky to visualize because on the euclidean space $\mathbb{R}^n$ the "reversed Gaussian" it is not normalizable, so we can only see it on the sphere.}
    \label{fig:rev_gaussian}
\end{figure} 


%APPROACH 1 (EASY, NOT FULLY PROBABILISTIC): 
The \textbf{evaluation} dataset $\mathcal{D}_E$ "interacts" with this distribution $p^c_{\mathcal{Z}}(\cdot|\mathcal{D}_A,\theta)$. Through the function $f_\theta$ it gives rise to a function (NOT a distribution) $p^c_{\mathcal{X}}$ on the data space for each class $c\in\mathcal{C}$ given by
\begin{equation}
    p^{c}_{\mathcal{X}}(x|\mathcal{D}_A,\theta)
    :=
    p^{c}_{\mathcal{Z}}(f_\theta(x)|\mathcal{D}_A,\theta)
    \qquad \forall x\in\mathcal{X}
\end{equation}
and the dataset likelihood-ish is defined by
\begin{equation}
    p(\mathcal{D}_E | \mathcal{D}_A, \theta)
    =
    \prod_{(x_e,c_e)\in\mathcal{D}_E}
    p^{c_e}_{\mathcal{X}}(x_e|\mathcal{D}_A,\theta).
\end{equation}
Expanding the RHS using \cref{eq:induced_distribution_definition}, we can write it as
\begin{equation}
    p(\mathcal{D}_E | \mathcal{D}_A, \theta)
    =
    \prod_{(x_e,c_e)\in\mathcal{D}_E}
    \left(
        \prod_{\substack{(x_a,c_a)\in\mathcal{D}_A \\ \text{s.t. } c_a = c_e}}
        p^{\shortrightarrow\shortleftarrow}(f_\theta(x_e)|x_a,\theta)
        \prod_{\substack{(x_a,c_a)\in\mathcal{D}_A \\ \text{s.t. } c_a\not= c_e}}
        p^{\shortleftarrow\shortrightarrow}(f_\theta(x_e)|x_a,\theta)
    \right)
\end{equation}

\iffalse
APPROACH 2 (NOT EASY, FULLY PROBABILISTIC): The \textbf{evaluation} dataset $\mathcal{D}_E$ "interacts" with this distribution $p^c_{\mathcal{Z}}(\cdot|\mathcal{D}_A,\theta)$. Through the function $f_\theta$ it gives rise to a distribution $p^c_{\mathcal{X}}$ on the data space for each class $c\in\mathcal{C}$ given by
\begin{equation}
    p^{c}_{\mathcal{X}}(x|\mathcal{D}_A,\theta)
    :=
    p^{c}_{\mathcal{Z}}(f_\theta(x)|\mathcal{D}_A,\theta)
    \det(J_x f_\theta(x))
\end{equation}
and the dataset likelihood is defined by
\begin{equation}
    p(\mathcal{D}_E | \mathcal{D}_A, \theta)
    =
    \prod_{(x_e,c_e)\in\mathcal{D}_E}
    p^{c_e}_{\mathcal{X}}(x_e|\mathcal{D}_A,\theta)
    =
    \prod_{(x_e,c_e)\in\mathcal{D}_E}
    p^{c_e}_{\mathcal{Z}}(f_\theta(x_e)|\mathcal{D}_A,\theta)
    \det(J_x f_\theta(x_e)).
\end{equation}
Expanding the RHS using \cref{eq:induced_distribution_definition}, we can write it as
\begin{align}
    p(\mathcal{D}_E | \mathcal{D}_A, \theta)
    &=
    \prod_{(x_e,c_e)\in\mathcal{D}_E}
    \left(
        \prod_{\substack{(x_a,c_a)\in\mathcal{D}_A \\ \text{s.t. } c_a = c_e}}
        p^{\shortrightarrow\shortleftarrow}(f_\theta(x_e)|x_a,\theta)
        \prod_{\substack{(x_a,c_a)\in\mathcal{D}_A \\ \text{s.t. } c_a\not= c_e}}
        p^{\shortleftarrow\shortrightarrow}(f_\theta(x_e)|x_a,\theta)
    \right) \\
    & \qquad \cdot
    \prod_{(x_e,c_e)\in\mathcal{D}_E}\det(J_x f_\theta(x_e))
\end{align}

NOW
\begin{itemize}
    \item APPROACH 1 is not fully probabilistic, what we derive is not really a likelihood on the data space
    \item APPROACH 2 is not equivalent to the classic non-probabilistic setting
\end{itemize}
BOTH ARE UNSATISFACTORY. WE NEED AN APPROACH 3...
\fi

\textbf{Problem (?)}: This view is nice since every single attractive/repulsive term $p^{\shortrightarrow\shortleftarrow}$ and $p^{\shortleftarrow\shortrightarrow}$ are proper distribution on the latent space, normalization constants are not dependent on $\theta$ and the math works smoothly. The non-nice part is that $p(\mathcal{D}_E | \mathcal{D}_A, \theta)$ is not a distribution, (so we can't call it likelihood). Yet it's a product of likelihood and thus the Laplace "precision" is a sum of proper precisions.



\subsection{Connecting the probabilistic and non-probabilistic settings}
Turns out that these two settings are indeed equivalent once we set $\mathcal{D}_E=\mathcal{D}_A$. The contrastive loss, as defined in \cref{eq:contrastive_definition}, is equal to the negative log likelihoods of attractive and repulsive term, evaluated on the latent representation $f_\theta(x_e)$ of the evaluation datapoint $x_e$
\begin{align}
    \text{contrastive}(\theta;x_e,c_e,x_a,c_a)
    & =
    \begin{cases}
        \frac{1}{2}\|f_\theta(x_e)-f_\theta(x_a)\|^2 & \text{if } c_e=c_a \\
        \max(-\frac{1}{2}\|f_\theta(x_e)-f_\theta(x_a)\|^2 + \frac{m}{2},0)  & \text{if } c_e\not=c_a
    \end{cases} \\
    & =
    \begin{cases}
        -\log p^{\shortrightarrow\shortleftarrow}(f_\theta(x_e)|x_a,\theta)
        + c^{\shortrightarrow\shortleftarrow}& \text{if } c_e=c_a \\
        -\log p^{\shortleftarrow\shortrightarrow}(f_\theta(x_e)|x_a,\theta)
        + c^{\shortleftarrow\shortrightarrow}& \text{if } c_e\not=c_a
    \end{cases},
\end{align}
where we highlight the symmetry of this term with respect to a switch of datapoints
\begin{equation}
    \text{contrastive}(\theta;x_e,c_e,x_a,c_a)
    =
    \text{contrastive}(\theta;x_a,c_a,x_e,c_e)
\end{equation}
which in turn implies the symmetry of the likelihood-ish with respect to a switch of datasets
\begin{equation}
    p(\mathcal{D}_E | \mathcal{D}_A, \theta)
    =
    p(\mathcal{D}_A | \mathcal{D}_E, \theta).
    %\qquad \forall \theta\in\Theta
\end{equation}

The dataset log-likelihood-ish is then %(AAA $\log p(\mathcal{D} | \mathcal{D}, \theta)$ is NOT the ideal notation)
\begin{align*}
    \log p&(\mathcal{D}_E | \mathcal{D}_A, \theta)\Big|_{\mathcal{D}_E=\mathcal{D}_A=\mathcal{D}} \\
    &=
    \sum_{(x_e,c_e)\in\mathcal{D}}
    \log p^{c_e}_{\mathcal{Z}}(f_\theta(x_e)|\mathcal{D},\theta) \\
    &= \sum_{(x_e,c_e)\in\mathcal{D}}
        \left(
        \sum_{\substack{(x_a,c_a)\in\mathcal{D} \\ \text{s.t. } c_a = c_e}}
        \log p^{\shortrightarrow\shortleftarrow}(f_\theta(x_e)|x_a,\theta)
        +
        \sum_{\substack{(x_a,c_a)\in\mathcal{D} \\ \text{s.t. } c_a\not= c_e}}
        \log p^{\shortleftarrow\shortrightarrow}(f_\theta(x_e)|x_a,\theta)
        \right) \\
     %={}& - \sum_{((x_e,c_e),(x_a,c_a))\in\mathcal{D}_E\times\mathcal{D}_A}
     %   \left(
     %   \delta_{c_a = c_e}
     %   \log p^{\shortrightarrow\shortleftarrow}(z|x_a,\theta)
     %   +
     %   \delta_{c_a \not= c_e}
     %   \log p^{\shortleftarrow\shortrightarrow}(z|x_a,\theta,m)
     %   \right)
     %   \Bigg|_{z=f_\theta(x_e)} \\
    &=
         \sum_{\substack{((x_e,c_e),(x_a,c_a))\in\mathcal{D}^2 \\ \text{s.t. } c_a = c_e}}
            \log p^{\shortrightarrow\shortleftarrow}(f_{\theta}(x_e)|x_a,\theta)
        +
         \sum_{\substack{((x_e,c_e),(x_a,c_a))\in\mathcal{D}^2 \\ \text{s.t. } c_a \not= c_e}}
            \log p^{\shortleftarrow\shortrightarrow}(f_{\theta}(x_e)|x_a,\theta) \\
    &= 
        \text{card}\{c_a=c_e\}c^{\shortrightarrow\shortleftarrow}
        +
        \text{card}\{c_a\not=c_e\}c^{\shortleftarrow\shortrightarrow}
        +\sum_{((x_e,c_e),(x_a,c_a))\in\mathcal{D}^2}
        -\text{contrastive}(\theta;x_e,c_e,x_a,c_a) \\
    &= 
        \text{card}\{c_a=c_e\}c^{\shortrightarrow\shortleftarrow}
        +
        \text{card}\{c_a\not=c_e\}c^{\shortleftarrow\shortrightarrow}
        -\text{loss}(\theta;\mathcal{D}).
\end{align*}
where $\text{card}\{c_a=c_e\}$ is the number of pairs of the same class (positive pairs) and $\text{card}\{c_a\not=c_e\}$ is the number of pairs of different classes (negative pairs). 

Notice that the normalization constants $c^{\shortrightarrow\shortleftarrow}$ and $c^{\shortleftarrow\shortrightarrow}$ are independent on $\theta$. Therefore, maximizing the likelihood is equivalent to minimizing the loss.

\fred{What does card stand for? This section is really nice and easy to understand!} \marco{Is the "cardinality of the set", not the best notation but the more compact I can think of.}

\subsection{Derivatives of the loss}
Having shown the equivalence of the two settings, we can use the easier notation of the non-probabilistic one in order to compute the derivatives.

First of all, the derivatives commute with the summation over datapoints
\begin{equation}
    \nabla_\theta\text{loss}(\theta;\mathcal{D})
    =
    \sum_{((x_e,c_e),(x_a,c_a))\in\mathcal{D}^2} \nabla_\theta\text{contrastive}(\theta;x_e,c_e,x_a,c_a)
\end{equation}
\begin{equation}
    \nabla^2_\theta\text{loss}(\theta;\mathcal{D})
    =
    \sum_{((x_e,c_e),(x_a,c_a))\in\mathcal{D}^2} \nabla^2_\theta\text{contrastive}(\theta;x_e,c_e,x_a,c_a)
\end{equation}
and so we can focus on a single pair contrastive term. It is useful to define an auxiliary function $l:\mathcal{Z}^2\rightarrow\mathbb{R}$ in order to keep the notation clear
\begin{align}
    l(z_1,z_2;b)
    :&=
    \begin{cases}
        \frac{1}{2}\|z_1 - z_2\|^2 & \text{if } b \\
        \max(-\frac{1}{2}\|z_1 - z_2\|^2 + \frac{m}{2},0)  & \text{if } \neg b
    \end{cases} \\
    &=
    \begin{cases}
        +\frac{1}{2}\|z_1 - z_2\|^2 & \text{if } b \\
        0 & \text{if } \neg b \text{ and } \|z_1 - z_2\|^2 > m \\
        -\frac{1}{2}\|z_1 - z_2\|^2 +\frac{m}{2}  & \text{if } \neg b\text{ and } \|z_1 - z_2\|^2 \leq m
    \end{cases}
\end{align}
which has derivatives
\begin{equation}
    \nabla_{z_1}l(z_1,z_2;b)
    =
    -\nabla_{z_2}l(z_1,z_2;b)
    =
    \begin{cases}
        z_1 - z_2 & \text{if } b \\
        0 & \text{if } \neg b \text{ and } \|z_1 - z_2\|^2 > m \\
        z_2 - z_1  & \text{if } \neg b\text{ and } \|z_1 - z_2\|^2 \leq m
    \end{cases}
\end{equation}
\begin{equation}
    \nabla^2_{z_1}l(z_1,z_2;b)
    =
    \nabla^2_{z_2}l(z_1,z_2;b)
    =
    \begin{cases}
        \mathbb{I}_\mathcal{Z} & \text{if } b \\
        0 & \text{if } \neg b \text{ and } \|z_1 - z_2\|^2 > m \\
        -\mathbb{I}_\mathcal{Z}  & \text{if } \neg b\text{ and } \|z_1 - z_2\|^2 \leq m
    \end{cases}
\end{equation}
\begin{equation}
    \nabla_{z_1}\nabla_{z_2}l(z_1,z_2;b)
    =
    \nabla_{z_2}\nabla_{z_1}l(z_1,z_2;b)
    =
    \begin{cases}
        -\mathbb{I}_\mathcal{Z} & \text{if } b \\
        0 & \text{if } \neg b \text{ and } \|z_1 - z_2\|^2 > m \\
        \mathbb{I}_\mathcal{Z}  & \text{if } \neg b\text{ and } \|z_1 - z_2\|^2 \leq m
    \end{cases}
\end{equation}


With this auxiliary function in place, we can write the contrastive as a composition of functions
\begin{equation}
    \text{contrastive}(\theta;x_e,c_e,x_a,c_a)
    =
    l(f_\theta(x_e),f_\theta(x_a);c_e=c_a)
\end{equation}
and compute the derivatives using the chain rule.

The \textbf{first order derivative} is
\begin{align*}
    \nabla_\theta&\text{contrastive}(\theta;x_e,c_e,x_a,c_a) \\
    & =
    \nabla_\theta l(f_\theta(x_e),f_\theta(x_a);c_e=c_a) \\
    & =
    \nabla_{\theta_1} l(f_{\theta_1}(x_e),f_\theta(x_a);c_e=c_a)\big|_{\theta_1=\theta}
    +
    \nabla_{\theta_2} l(f_\theta(x_e),f_{\theta_2}(x_a);c_e=c_a)\big|_{\theta_2=\theta} \\
    & =
    J_\theta f_\theta(x_e)^\top \nabla_{z} l(z,f_\theta(x_a);c_e=c_a)\big|_{z=f_\theta(x_e)}
    +
    J_\theta f_\theta(x_a)^\top \nabla_{z} l(f_\theta(x_e),z;c_e=c_a)\big|_{z=f_\theta(x_a)} \\
    & =
    \begin{cases}
        \begin{pmatrix}
        J_\theta f_\theta(x_e) \\ -J_\theta f_\theta(x_a)
        \end{pmatrix}^\top (f_\theta(x_e)-f_\theta(x_a))
        & \text{if } c_e=c_a \\
        0 
        & \text{if } c_e\not=c_a \text{ and } \|f_\theta(x_e) - f_\theta(x_a)\|^2 > m \\
        \begin{pmatrix}
        J_\theta f_\theta(x_e) \\ -J_\theta f_\theta(x_a)
        \end{pmatrix}^\top (f_\theta(x_a)-f_\theta(x_e)) 
        & \text{if } c_e\not=c_a \text{ and } \|f_\theta(x_e) - f_\theta(x_a)\|^2 \leq m
    \end{cases}
\end{align*}

The \textbf{second order derivative} (neglecting $\nabla^2_\theta f$ in the chain rule in the third equality) is
\begin{align*}
    \nabla^2_\theta&\text{contrastive}(\theta;x_e,c_e,x_a,c_a) \\
    & =
    \nabla^2_\theta l(f_\theta(x_e),f_\theta(x_a);c_e=c_a) \\
    % LINE 2
    & =
    \nabla_\theta
    \left(
    \nabla_{\theta_1} l(f_{\theta_1}(x_e),f_\theta(x_a);c_e=c_a)\big|_{\theta_1=\theta}
    +
    \nabla_{\theta_2} l(f_\theta(x_e),f_{\theta_2}(x_a);c_e=c_a)\big|_{\theta_2=\theta} 
    \right)\\
    % LINE 3
    & =
    \nabla^2_{\theta_1} l(f_{\theta_1}(x_e),f_\theta(x_a);c_e=c_a)\big|_{\theta_1=\theta}
    +
    \nabla_{\theta_2}\nabla_{\theta_1} l(f_\theta(x_e),f_{\theta_2}(x_a);c_e=c_a)\big|_{\theta_1=\theta_2=\theta} \\
    &\qquad +
    \nabla_{\theta_1}\nabla_{\theta_2} l(f_\theta(x_e),f_{\theta_2}(x_a);c_e=c_a)\big|_{\theta_1=\theta_2=\theta} 
    +
    \nabla^2_{\theta_2} l(f_\theta(x_e),f_{\theta_2}(x_a);c_e=c_a)\big|_{\theta_2=\theta} \\
    % LINE 4
    & =
    J_\theta f_\theta(x_e)^\top \nabla^2_{z_1} l(z_1,z_2;c_e=c_a)\big|_{z_1=f_\theta(x_e),z_2=f_\theta(x_a)} J_\theta f_\theta(x_e)\\
    &\qquad +
    J_\theta f_\theta(x_a)^\top \nabla_{z_2}\nabla_{z_1} l(z_1,z_2;c_e=c_a)\big|_{z_1=f_\theta(x_e),z_2=f_\theta(x_a)} J_\theta f_\theta(x_e)\\
    &\qquad+
    J_\theta f_\theta(x_e)^\top \nabla_{z_1}\nabla_{z_2} l(z_1,z_2;c_e=c_a)\big|_{z_1=f_\theta(x_e),z_2=f_\theta(x_a)} J_\theta f_\theta(x_a)\\
    &\qquad+
    J_\theta f_\theta(x_a)^\top \nabla^2_{z_2} l(z_1,z_2;c_e=c_a)\big|_{z_1=f_\theta(x_e),z_2=f_\theta(x_a)} J_\theta f_\theta(x_a) \\
    % LINE 5
    & =
    \begin{cases}
        \begin{pmatrix}
        J_\theta f_\theta(x_e) \\ J_\theta f_\theta(x_a)
        \end{pmatrix}^\top 
        \begin{pmatrix}
        2 & -2 \\ -2 & 2
        \end{pmatrix}
        \begin{pmatrix}
        J_\theta f_\theta(x_e) \\ J_\theta f_\theta(x_a)
        \end{pmatrix}
        & \text{if } c_e=c_a \\
        0 
        & \text{if } c_e\not=c_a \text{ and } \|f_\theta(x_e) - f_\theta(x_a)\|^2 > m \\
        \begin{pmatrix}
        J_\theta f_\theta(x_e) \\ J_\theta f_\theta(x_a)
        \end{pmatrix}^\top
        \begin{pmatrix}
        -2 & 2 \\ 2 & -2
        \end{pmatrix}
        \begin{pmatrix}
        J_\theta f_\theta(x_e) \\ J_\theta f_\theta(x_a)
        \end{pmatrix}
        & \text{if } c_e\not=c_a \text{ and } \|f_\theta(x_e) - f_\theta(x_a)\|^2 \leq m
    \end{cases}
\end{align*}

Then we can write a closed expression for the hessian of the loss, assuming $f$ to be linear in $\theta$
\begin{align}
    \nabla^2_\theta \text{loss}(\theta;\mathcal{D})
    & =
    \sum_{\substack{((x_e,c_e),(x_a,c_a))\in\mathcal{D}^2 \\ \text{s.t. } c_a = c_e}}
        \begin{pmatrix}
        J_\theta f_\theta(x_e) \\ J_\theta f_\theta(x_a)
        \end{pmatrix}^\top 
        \begin{pmatrix}
        2 & -2 \\ -2 & 2
        \end{pmatrix}
        \begin{pmatrix}
        J_\theta f_\theta(x_e) \\ J_\theta f_\theta(x_a)
        \end{pmatrix} \\
    & \qquad +
    \sum_{\substack{((x_e,c_e),(x_a,c_a))\in\mathcal{D}^2 \\ \text{s.t. } c_a\not= c_e \text{ and}\\ \|f_\theta(x_e) - f_\theta(x_a)\|^2 \leq m}}
        \begin{pmatrix}
        J_\theta f_\theta(x_e) \\ J_\theta f_\theta(x_a)
        \end{pmatrix}^\top
        \begin{pmatrix}
        -2 & 2 \\ 2 & -2
        \end{pmatrix}
        \begin{pmatrix}
        J_\theta f_\theta(x_e) \\ J_\theta f_\theta(x_a)
        \end{pmatrix}
\end{align}


\subsection{Positive definiteness}
We can further analyze and exploit the structure of this hessian. The loss term for positive pairs $\begin{pmatrix} 2 & -2 \\ -2 & 2\end{pmatrix}$ has eigenvalues $0$ and $4$ with eigenvectors $(1,1)$ and $(1,-1)$ respectively. Thus is a positive semidefinite matrix, and so it remains when we multiply from both left and right by the same matrix.\\
The opposite holds true for the negative pairs: the loss term $\begin{pmatrix} -2 & 2 \\ 2 & -2\end{pmatrix}$ has the same eigenvectors, but with eigenvalues $0$ and $-4$. Thus it is negative semidefinite.

Is $\nabla^2_\theta \text{loss}(\theta;\mathcal{D})$ positive definite? Mh

\textbf{Solution A}: Easy solution is to neglect all the negative pairs inside the margin. In this way, the positive semidefiniteness of the matrix $\begin{pmatrix} 2 & -2 \\ -2 & 2\end{pmatrix}$ implies the positive semidefiniteness of the loss. But neglecting the negative terms is not nice.

\textbf{Solution B}: We can neglect the crossed terms and place a $\frac{1}{|\mathcal{C}|-1}$ discount term in front of the negative term of the loss. With these assumption we have
\begin{equation*}
    \text{contrastive}^\text{weighted}(\theta;x_e,c_e,x_a,c_a)
    =
    \begin{cases}
        \frac{1}{2}\|f_\theta(x_e)-f_\theta(x_a)\|^2 & \text{if } c_e=c_a \\
        \frac{1}{|\mathcal{C}|-1}\frac{1}{2}\max(-\|f_\theta(x_e)-f_\theta(x_a)\|^2 + m,0)  & \text{if } c_e\not=c_a
    \end{cases}
\end{equation*}
and
\begin{align*}
    \nabla^2_\theta & \text{loss}^\text{weighted}(\theta;\mathcal{D})\\
    & =
    \sum_{\substack{((x_e,c_e),(x_a,c_a))\in\mathcal{D}^2 \\ \text{s.t. } c_a = c_e}}
        \begin{pmatrix}
        J_\theta f_\theta(x_e) \\ J_\theta f_\theta(x_a)
        \end{pmatrix}^\top 
        \begin{pmatrix}
        2 & -2 \\ -2 & 2
        \end{pmatrix}
        \begin{pmatrix}
        J_\theta f_\theta(x_e) \\ J_\theta f_\theta(x_a)
        \end{pmatrix} \\
    & \qquad +
    \frac{1}{|\mathcal{C}|-1}
    \sum_{\substack{((x_e,c_e),(x_a,c_a))\in\mathcal{D}^2 \\ \text{s.t. } c_a\not= c_e \text{ and}\\ \|f_\theta(x_e) - f_\theta(x_a)\|^2 \leq m}}
        \begin{pmatrix}
        J_\theta f_\theta(x_e) \\ J_\theta f_\theta(x_a)
        \end{pmatrix}^\top
        \begin{pmatrix}
        -2 & 2 \\ 2 & -2
        \end{pmatrix}
        \begin{pmatrix}
        J_\theta f_\theta(x_e) \\ J_\theta f_\theta(x_a)
        \end{pmatrix} \\
    & \approx
    \sum_{\substack{((x_e,c_e),(x_a,c_a))\in\mathcal{D}^2 \\ \text{s.t. } c_a = c_e}}
        \begin{pmatrix}
        J_\theta f_\theta(x_e) \\ J_\theta f_\theta(x_a)
        \end{pmatrix}^\top 
        \begin{pmatrix}
        2 & 0 \\ 0 & 2
        \end{pmatrix}
        \begin{pmatrix}
        J_\theta f_\theta(x_e) \\ J_\theta f_\theta(x_a)
        \end{pmatrix} \\
    & \qquad +
    \frac{1}{|\mathcal{C}|-1}
    \sum_{\substack{((x_e,c_e),(x_a,c_a))\in\mathcal{D}^2 \\ \text{s.t. } c_a\not= c_e \text{ and}\\ \|f_\theta(x_e) - f_\theta(x_a)\|^2 \leq m}}
        \begin{pmatrix}
        J_\theta f_\theta(x_e) \\ J_\theta f_\theta(x_a)
        \end{pmatrix}^\top
        \begin{pmatrix}
        -2 & 0 \\ 0 & -2
        \end{pmatrix}
        \begin{pmatrix}
        J_\theta f_\theta(x_e) \\ J_\theta f_\theta(x_a)
        \end{pmatrix} \\
    & =
    \sum_{\substack{((x_e,c_e),(x_a,c_a))\in\mathcal{D}^2 \\ \text{s.t. } c_a = c_e}}
        2J_\theta f_\theta(x_e)^\top
        J_\theta f_\theta(x_e)
    +
    \frac{1}{|\mathcal{C}|-1}
    \sum_{\substack{((x_e,c_e),(x_a,c_a))\in\mathcal{D}^2 \\ \text{s.t. } c_a\not= c_e \text{ and}\\ \|f_\theta(x_e) - f_\theta(x_a)\|^2 \leq m}}
        -2J_\theta f_\theta(x_e)^\top
        J_\theta f_\theta(x_e) \\
    & \qquad +
    \sum_{\substack{((x_e,c_e),(x_a,c_a))\in\mathcal{D}^2 \\ \text{s.t. } c_a = c_e}}
        2J_\theta f_\theta(x_a)^\top
        J_\theta f_\theta(x_a)
    +
    \frac{1}{|\mathcal{C}|-1}
    \sum_{\substack{((x_e,c_e),(x_a,c_a))\in\mathcal{D}^2 \\ \text{s.t. } c_a\not= c_e \text{ and}\\ \|f_\theta(x_e) - f_\theta(x_a)\|^2 \leq m}}
        -2J_\theta f_\theta(x_a)^\top
        J_\theta f_\theta(x_a) \\
    & =
    4 \sum_{(x_a,c_a)\in\mathcal{D}}
        J_\theta f_\theta(x_a)^\top
        J_\theta f_\theta(x_a)
        \left(
        \sum_{\substack{(x_e,c_e)\in\mathcal{D} \\ \text{s.t. } c_a = c_e}}
        1
        -
        \sum_{\substack{(x_e,c_e)\in\mathcal{D} \\ \text{s.t. } c_a \not= c_e \text{ and}\\ \|f_\theta(x_e) - f_\theta(x_a)\|^2 \leq m}}
        \frac{1}{|\mathcal{C}|-1}
        \right) \\
    & =
    4 
    \left(|c_a=c_e| - \frac{|c_a\not=c_e \text{ in margin}|}{|\mathcal{C}|-1}
    \right)
    \sum_{(x,c)\in\mathcal{D}}
        J_\theta f_\theta(x)^\top
        J_\theta f_\theta(x)
\end{align*}
That is guaranteed to be positive semidefinite by noticing that \begin{equation}
\frac{|c_a=c_e|}{|c_a\not=c_e \text{ in margin}|}\leq\frac{|c_a=c_e|}{|c_a\not=c_e|}=\frac{1}{|\mathcal{C}|-1}.
\end{equation}

But neglecting the crossed terms is not super nice (still better that Solution A). It can be reasoned by assuming that, in the two occurrence of $\theta$ in the loss (one for ancor, one for evaluation) one of the two is fixed, and we derive only with respect to the other one.

N.B. This is weird but coherent with the classic metric learning. In fact fixing or not fixing does not change the first order derivative.



\textbf{Solution C}: Neglecting nothing! (SPOILER: Not working, yet) Let's try a tricky approach. Perform a Hadamard transformation by defining
\begin{equation}
    J^+(x_e,x_a) 
    := J_\theta f_\theta(x_e) + J_\theta f_\theta(x_a)
\end{equation}
\begin{equation}
    J^-(x_e,x_a) 
    := J_\theta f_\theta(x_e) - J_\theta f_\theta(x_a)
\end{equation}
that imply
\begin{equation}
    J_\theta f_\theta(x_e)
    = \frac{1}{2} (J^+(x_e,x_a) + J^-(x_e,x_a))
\end{equation}
\begin{equation}
    J_\theta f_\theta(x_a)
    = \frac{1}{2} (J^+(x_e,x_a) - J^-(x_e,x_a))
\end{equation}

And we can take advantage of the anti-symmetry 
\begin{equation}
    J^-(x_1,x_2) = - J^-(x_2,x_1)
    \qquad
    \forall x_1,x_2
\end{equation}
and of the triangular relationship
\begin{equation}
    J^-(x_1,x_2) + J^-(x_2,x_3) = J^-(x_1,x_3)
    \qquad
    \forall x_1,x_2,x_3
\end{equation}
\iffalse
that together with Cauchy gives (but this is false aaaaa)
\begin{align*}
    J^-(x_1,x_2)^\top J^-(x_1,x_2) + J^-(x_2,x_3)^\top J^-(x_2,x_3) 
    &\leq
    2
    \left(J^-(x_1,x_2)+J^-(x_2,x_3)\right)^\top
    \left(J^-(x_1,x_2)+J^-(x_2,x_3)\right) \\
    &= 
    2J^-(x_1,x_3)^\top J^-(x_1,x_3)
\end{align*}
the idea now is to use this equation to prove the positive definiteness, specifically using $x_1$ and $x_3$ in the same class (and their attractive term) to eat all the $x_2$ in different classes (and their repulsive terms).
\fi

Then we can rewrite the hessian as
\begin{align*}
    \nabla^2_\theta & \text{loss}^\text{weighted}(\theta;\mathcal{D})\\
    & =
    \sum_{\substack{((x_e,c_e),(x_a,c_a))\in\mathcal{D}^2 \\ \text{s.t. } c_a = c_e}}
        \begin{pmatrix}
        J_\theta f_\theta(x_e) \\ J_\theta f_\theta(x_a)
        \end{pmatrix}^\top 
        \begin{pmatrix}
        2 & -2 \\ -2 & 2
        \end{pmatrix}
        \begin{pmatrix}
        J_\theta f_\theta(x_e) \\ J_\theta f_\theta(x_a)
        \end{pmatrix} \\
    & \qquad +
    \frac{1}{|\mathcal{C}|-1}
    \sum_{\substack{((x_e,c_e),(x_a,c_a))\in\mathcal{D}^2 \\ \text{s.t. } c_a\not= c_e \text{ and}\\ \|f_\theta(x_e) - f_\theta(x_a)\|^2 \leq m}}
        \begin{pmatrix}
        J_\theta f_\theta(x_e) \\ J_\theta f_\theta(x_a)
        \end{pmatrix}^\top
        \begin{pmatrix}
        -2 & 2 \\ 2 & -2
        \end{pmatrix}
        \begin{pmatrix}
        J_\theta f_\theta(x_e) \\ J_\theta f_\theta(x_a)
        \end{pmatrix} \\
    % new line
    & =
    \frac{1}{2}
    \sum_{\substack{((x_e,c_e),(x_a,c_a))\in\mathcal{D}^2 \\ \text{s.t. } c_a = c_e}}
        \begin{pmatrix}
        J^+(x_e,x_a) + J^-(x_e,x_a) \\ J^+(x_e,x_a) - J^-(x_e,x_a)
        \end{pmatrix}^\top 
        \begin{pmatrix}
        1 & -1 \\ -1 & 1
        \end{pmatrix}
        \begin{pmatrix}
        J^+(x_e,x_a) + J^-(x_e,x_a) \\ J^+(x_e,x_a) - J^-(x_e,x_a)
        \end{pmatrix} \\
    & \qquad +
    \frac{1}{2}
    \frac{1}{|\mathcal{C}|-1}
    \sum_{\substack{((x_e,c_e),(x_a,c_a))\in\mathcal{D}^2 \\ \text{s.t. } c_a\not= c_e \text{ and}\\ \|f_\theta(x_e) - f_\theta(x_a)\|^2 \leq m}}
        \begin{pmatrix}
        J^+(x_e,x_a) + J^-(x_e,x_a) \\ J^+(x_e,x_a) - J^-(x_e,x_a)
        \end{pmatrix}^\top
        \begin{pmatrix}
        -1 & 1 \\ 1 & -1
        \end{pmatrix}
        \begin{pmatrix}
        J^+(x_e,x_a) + J^-(x_e,x_a) \\ J^+(x_e,x_a) - J^-(x_e,x_a)
        \end{pmatrix} \\
    % new line
    & =
    \frac{1}{2}
    \sum_{\substack{((x_e,c_e),(x_a,c_a))\in\mathcal{D}^2 \\ \text{s.t. } c_a = c_e}}
        \begin{pmatrix}
        J^-(x_e,x_a) \\ - J^-(x_e,x_a)
        \end{pmatrix}^\top 
        \begin{pmatrix}
        1 & -1 \\ -1 & 1
        \end{pmatrix}
        \begin{pmatrix}
        J^-(x_e,x_a) \\ - J^-(x_e,x_a)
        \end{pmatrix} \\
    & \qquad +
    \frac{1}{2}
    \frac{1}{|\mathcal{C}|-1}
    \sum_{\substack{((x_e,c_e),(x_a,c_a))\in\mathcal{D}^2 \\ \text{s.t. } c_a\not= c_e \text{ and}\\ \|f_\theta(x_e) - f_\theta(x_a)\|^2 \leq m}}
        \begin{pmatrix}
        J^-(x_e,x_a) \\ - J^-(x_e,x_a)
        \end{pmatrix}^\top
        \begin{pmatrix}
        -1 & 1 \\ 1 & -1
        \end{pmatrix}
        \begin{pmatrix}
        J^-(x_e,x_a) \\ - J^-(x_e,x_a)
        \end{pmatrix} \\
    % new line
    & =
    2
    \sum_{\substack{((x_e,c_e),(x_a,c_a))\in\mathcal{D}^2 \\ \text{s.t. } c_a = c_e}}
        \underbrace{
        J^-(x_e,x_a)^\top J^-(x_e,x_a)
        }_{\text{pos semidefinite}}
    +
    \frac{2}{|\mathcal{C}|-1}
    \sum_{\substack{((x_e,c_e),(x_a,c_a))\in\mathcal{D}^2 \\ \text{s.t. } c_a\not= c_e \text{ and}\\ \|f_\theta(x_e) - f_\theta(x_a)\|^2 \leq m}}
        \underbrace{
        -J^-(x_e,x_a)^\top J^-(x_e,x_a)
        }_{\text{neg semidefinite}} \\
    % new line
    & =
    2
    \sum_{c\in\mathcal{C}}
    \left(
    \sum_{(x_e,x_a)\in\mathcal{D}_c^2}
        J^-(x_e,x_a)^\top J^-(x_e,x_a)
    +
    \frac{1}{|\mathcal{C}|-1}
    \sum_{\substack{c'\in\mathcal{C} \\ \text{s.t. } c'\not=c}}
    \sum_{\substack{(x_e,x_a)\in\mathcal{D}_{c}\times\mathcal{D}_{c'}  \\ \text{s.t. }  \\ \|f_\theta(x_e) - f_\theta(x_a)\|^2 \leq m}}
        -J^-(x_e,x_a)^\top J^-(x_e,x_a)
    \right)
\end{align*}
\emph{Intuitively} this matrix will fail in being positive definite in the case when there exists a direction $v_\theta$ such that moving $\theta\rightarrow\theta+v_\theta$ induces a low internal average velocity in each class, but at the same time induces an high relative velocity between different classes. This, locally speaking, is a divergent behaviour, and will lead to undefined uncertainty. 

STILL if such direction exists, then the gradient will have positive component in that direction and it won't be 0. Does the invert implication holds??? i.e. if the gradient is small enough, then there shouldn't exist bad behaved directions. We can write the gradient as
\begin{align*}
    \nabla_\theta & \text{loss}^\text{weighted}(\theta;\mathcal{D})\\
    & =
    \sum_{c\in\mathcal{C}}
    \left(
    2
    \sum_{(x_e,x_a)\in\mathcal{D}_c^2}
        \underbrace{
        J^-(x_e,x_a)
        (f_\theta(x_e)-f_\theta(x_a))
        }_{\text{weighted average internal $c$ velocity}}
    +
    \frac{1}{|\mathcal{C}|-1}
    \sum_{\substack{c'\in\mathcal{C} \\ \text{s.t. } c'\not=c}}
    \sum_{\substack{(x_e,x_a)\in\mathcal{D}_{c}\times\mathcal{D}_{c'}  \\ \text{s.t. }  \\ \|f_\theta(x_e) - f_\theta(x_a)\|^2 \leq m}}
        \underbrace{
        -J^-(x_e,x_a)
        (f_\theta(x_e)-f_\theta(x_a))
        }_{\text{weighted average interclass $c/c'$ velocity}}
    \right)
\end{align*}




\subsection{Metric learning}
With the probabilistic interpretation we can define the dataset likelihood, conditioned to some parameter $\theta$, as
\begin{equation}
    p(\mathcal{D}|\theta) 
    =
    p(\mathcal{D}_E | \mathcal{D}_A, \theta)\Big|_{\mathcal{D}_E=\mathcal{D}_A=\mathcal{D}}
\end{equation}
which in turn following Bayes rule defines the parameter likelihood, conditioned to the dataset, as
\begin{equation}
    p(\theta|\mathcal{D})
    =
    \frac{p(\mathcal{D}|\theta) p(\theta)}{p(\mathcal{D})}
\end{equation}

The aim of metric learning is to maximise such likelihood with respect to the parameter $\theta$, specifically it aims at finding the Maximum A Posteriori
\begin{equation}
    \theta^{\text{MAP}} \in \argmax_{\theta\in\Theta} p(\theta|\mathcal{D}).
\end{equation}
As shown before, finding Maximum A Posteriori is equivalent to find the minimum of the loss. 
More generally in our Bayesian setting we do not seek only of a maxima, but we seek for an expression of the whole distribution $p(\theta|\mathcal{D})$. We do that by maximizing the dataset likelihood $p(\mathcal{D})$ by integrating out $\theta$ with $p(\mathcal{D})=\E_{\theta\sim q}[p(\mathcal{D} | \theta)]$. This maximization is then defined by
\begin{align}
    q^*(\theta)
    :=
    p^*(\theta|\mathcal{D})
    \in 
    \argmax_{p(\theta|\mathcal{D})\in\mathcal{G}(\Theta)} 
        \E_{\theta\sim p(\theta|\mathcal{D})}
        [p(\mathcal{D} | \theta)]
\end{align}

Notice that, limited by the ability to parametrize distributions, we aim at finding such maxima on $q$ over only some subspace of distributions on $\Theta$. Specifically we resctrict ourselves to the space of Gaussians $\mathcal{G}(\Theta)\subset\Delta(\Theta)$. This is a strong assumption since, in principle, there is no guarantees of $p(\theta|\mathcal{D})$ being Gaussian, even approximately. Nonetheless forcing this approximation to be centered in $\theta^{\text{MAP}}$ (as Laplace Post-Hoc does) is a further assumption with no guarantees of holding true. This is why we should always opt for online Laplace over Laplace post-hoc.

%\textbf{Post-hoc no-sense warning:} With these two definitions it is NOT guaranteed that the mode of $q^*$ is $\theta^{\text{MAP}}$. So one may wonder if Laplace post-hoc does really makes sense? (Laplace Post-Hoc, by definition, centers its gaussian $q^*$ in $\theta^{\text{MAP}}$)

%Wait. We need to be more careful. With this definition, the optimal Gaussian $q*$ would be a degenerate Gaussian with zero variance, centered in $\theta^{\text{MAP}}$


\subsection{Laplace post-hoc}
The Bayes rule
\begin{equation}
    p(\theta|\mathcal{D})
    =
    \frac{p(\mathcal{D}|\theta) p(\theta)}{p(\mathcal{D})}
\end{equation}
implies that
\begin{equation}
    \nabla^2_\theta \log p(\theta|\mathcal{D})
    =
    \nabla^2_\theta \log p(\mathcal{D}|\theta) 
    +
    \nabla^2_\theta \log p(\theta).
\end{equation}

Assuming a Gaussian prior $p(\theta)\sim\mathcal{N}(\theta|0,\sigma_{\text{prior}}\mathbb{I})$ implies $\nabla^2_\theta \log p(\theta)=-\sigma_{\text{prior}}^{-1}\mathbb{I}$ and we have
\begin{equation}
    \nabla^2_\theta \log p(\theta|\mathcal{D})
    =
    -\nabla^2_\theta \text{loss}(\theta;\mathcal{D}) 
    -
    \sigma_{\text{prior}}^{-1}\mathbb{I}.
\end{equation}
Thus, we have two options:
\begin{itemize}
    \item IF $p(\theta|\mathcal{D})$ is a Gaussian it holds $\forall \theta^*\in\Theta$
\begin{equation}
    p(\theta|\mathcal{D})
    \sim
    \mathcal{N}(\theta|\mu=\theta^{\text{MAP}},\Sigma = (\nabla^2_\theta \text{loss}(\theta^*;\mathcal{D}) 
    +
    \sigma_{\text{prior}}^{-1}\mathbb{I})^{-1})
\end{equation}

    \item ELSE we can do a second order Taylor approximation of $\log p(\theta|\mathcal{D})$ around $\theta^{\text{MAP}}$ and we have the approximation
\begin{equation}
    p(\theta|\mathcal{D})
    \sim
    \mathcal{N}(\theta|\mu=\theta^{\text{MAP}},\Sigma = (\nabla^2_\theta \text{loss}(\theta^{\text{MAP}};\mathcal{D}) 
    +
    \sigma_{\text{prior}}^{-1}\mathbb{I})^{-1})
\end{equation}
\end{itemize}


\subsection{Laplace online}
At every step $t$ we have some Gaussian on the parameter space
\begin{equation}
    q^t(\theta)
    \sim
    \mathcal{N}(\theta|\mu=\theta_t,\Sigma=(H_t)^{-1})
\end{equation}
Where the values $\theta_t$ and $H_t$ are iteratively defined as
\begin{equation}\label{eq:updaterule_theta_point}
    \theta_{t+1}
    =
    \theta_t
    +
    \lambda
    \nabla_\theta \text{loss}(\theta_t;\mathcal{D}) 
    \qquad
    \theta_0 = \mu_{\text{prior}}
\end{equation}
and
\begin{equation}\label{eq:updaterule_precision_point}
    H_{t+1}
    =
    (1-\alpha) H_t
    +
    \nabla^2_\theta \text{loss}(\theta_t;\mathcal{D}) 
    \qquad
    H_0 = \sigma_{\text{prior}}^{-1}\mathbb{I}
\end{equation}
For some learning rate $\lambda$ and memory factor $\alpha$. This means that $q^0(\theta)$ is actually the prior distribution, and the we update it with first and second order derivatives of the loss. The updates can be improved by computing the derivatives not only in the sigle point $\theta_t$, but rather on expected value with $\theta$ following the distribution $q^t$. This leads to the update rules
\begin{equation}\label{eq:updaterule_theta_expected}
    \theta_{t+1}
    =
    \theta_t
    +
    \lambda
    \mathbb{E}_{\theta\sim q^t(\theta)}
    [\nabla_\theta \text{loss}(\theta;\mathcal{D}) 
    ]
    \qquad
    \theta_0 = \mu_{\text{prior}}
\end{equation}
and
\begin{equation}\label{eq:updaterule_precision_expected}
    H_{t+1}
    =
    (1-\alpha) H_t
    +
    \mathbb{E}_{\theta\sim q^t(\theta)}
    [\nabla^2_\theta \text{loss}(\theta;\mathcal{D}) 
    ]
    \qquad
    H_0 = \sigma_{\text{prior}}^{-1}\mathbb{I}
\end{equation}

Rule \cref{eq:updaterule_precision_expected} take into account third order dependencies (take we assume to be neglectable) and, not less importantly, it is super expensive to compute. Therefor we actually use update rules \cref{eq:updaterule_theta_expected} and \cref{eq:updaterule_precision_point} for $\theta_t$ and $H_t$ respectively. 
